# Supplementary material for: An Evaluation of Anomaly Detection and Diagnosis in Multivariate Time Series
Source: arXiv:2109.11428 source file (2021-09-23)
Supplement: Supplementary file 1 [file scoring_thres_params.tex]

% Please add the following required packages to your document preamble:
% \usepackage{booktabs}
\begin{table*}
\centering
\caption{Hyperparameters for scoring and thresholding functions.}
\label{tab:scoring_thres_params}
% \resizebox{\textwidth}{!}{%
\begin{tabular}{@{}llllllll@{}}
\toprule
Method               & Hyperparameter        & DAMADICS & SWaT & WADI & MSL  & SMAP & SMD  \\ \midrule
Gauss-D,   Gauss-D-K & $W'$ & 10       & 10   & 10   & 10   & 10   & 10   \\
 &
  $W$ &
  $10^5$ &
  $10^5$ &
  $10^5$ &
  2000 &
  2000 &
  $10^4$ \\
Gauss-D-K            & $\sigma_k$  & 120      & 120  & 120  & 10   & 10   & 10   \\ \bottomrule
% POT,   DSPOT &
%   $q$ &
%   $10^{-3}$ &
%   $10^{-3}$ &
%   $10^{-3}$ &
%   $10^{-3}$ &
%   $10^{-3}$ &
%   $10^{-3}$ \\
%                      &  percentile    & 0.98     & 0.98 & 0.98 & 0.98 & 0.98 & 0.98 \\
% DSPOT                & depth                 & 120      & 7500 & 7500 & 2100 & 2100 & 7500 \\
% Tail P &
%   $p$ &
%   $10^{-6}$ &
%   $10^{-6}$ &
%   $10^{-6}$ &
%   $10^{-6}$ &
%   $10^{-6}$ &
%   $10^{-6}$ \\ \bottomrule
\end{tabular}
% }
\end{table*}
